# Supplementary material for: A Radiative Transfer Framework for Spatially-Correlated Materials
Source: arXiv:1805.02651 source file (2018-05-07)

---

---

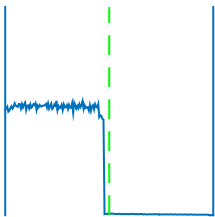

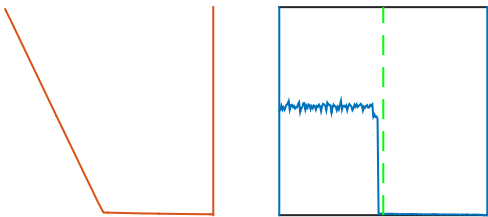

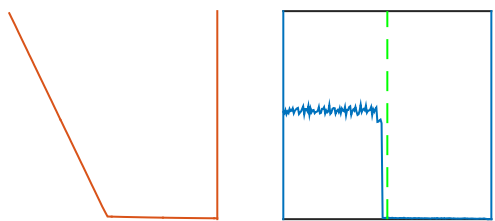

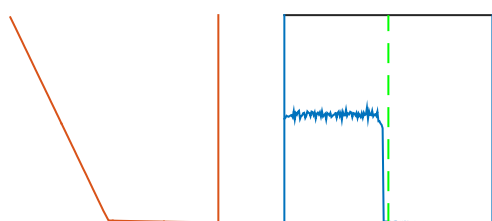

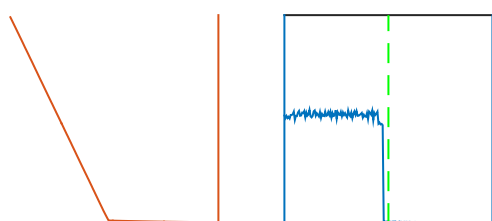

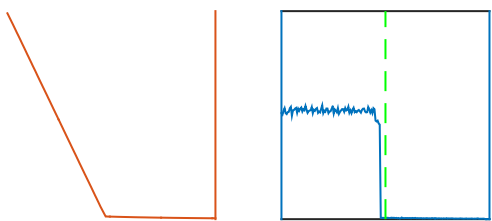

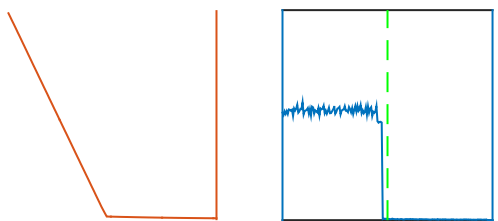



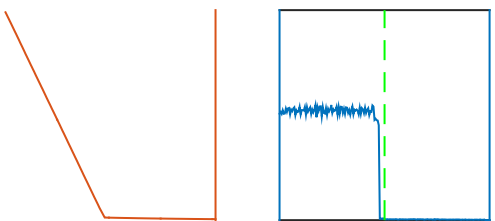

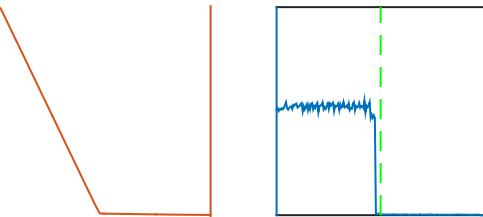

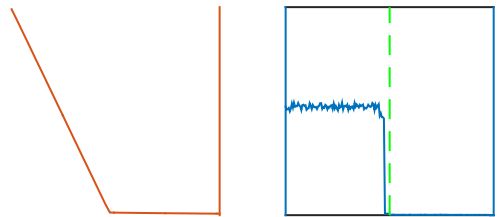

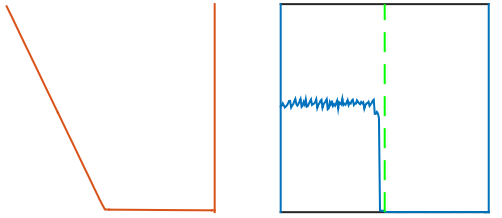



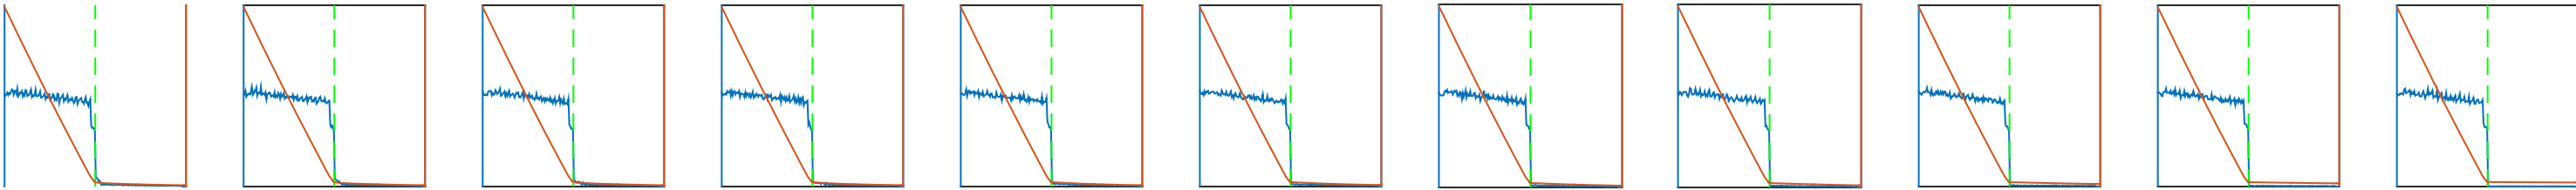

\_\_\_\_\_

\_\_\_\_\_

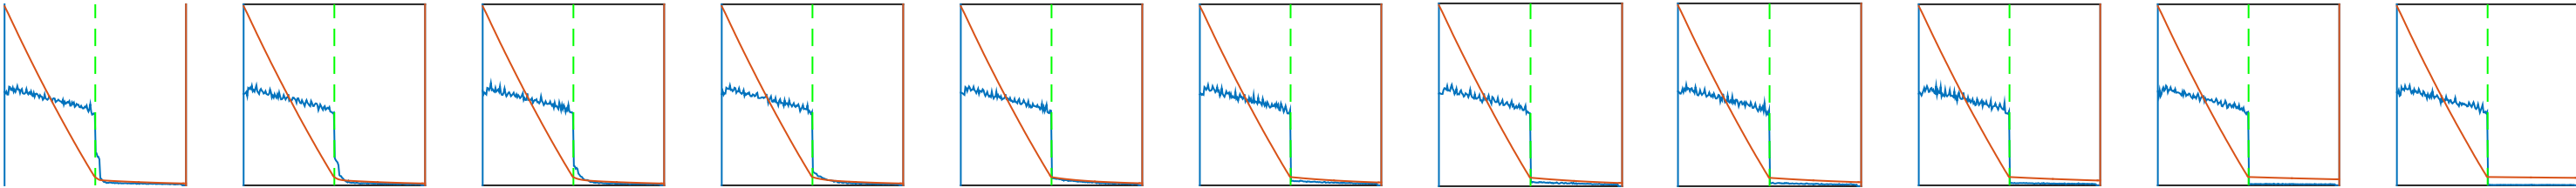

\_\_\_\_\_

\_\_\_\_\_

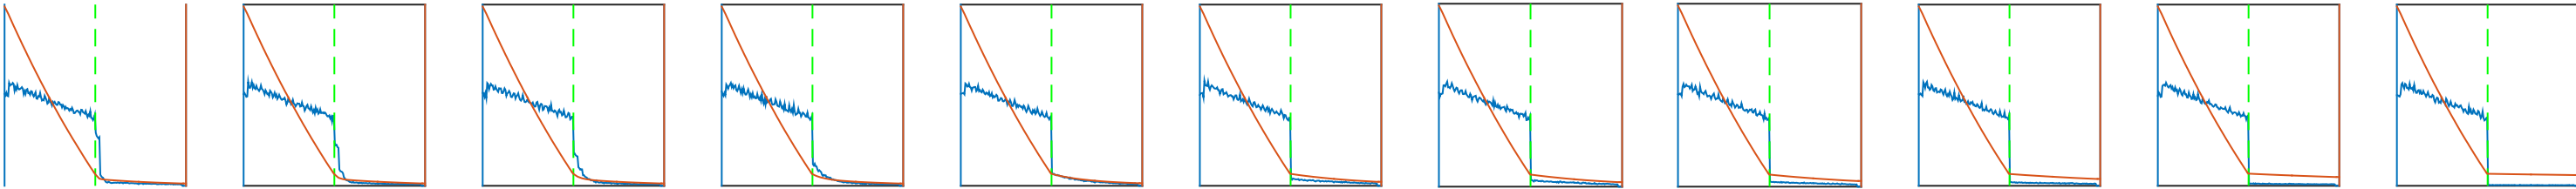

\_\_\_\_\_

\_\_\_\_\_



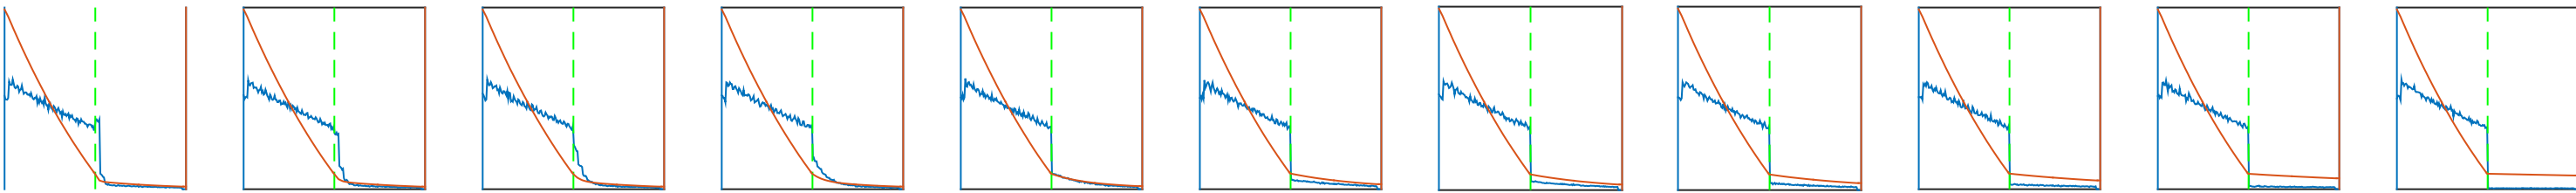

\_\_\_\_\_

\_\_\_\_\_

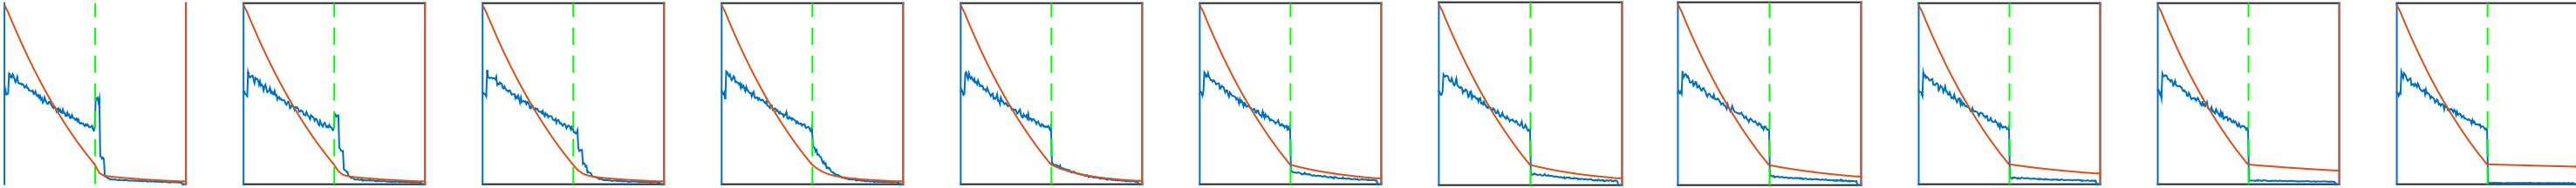

---

---

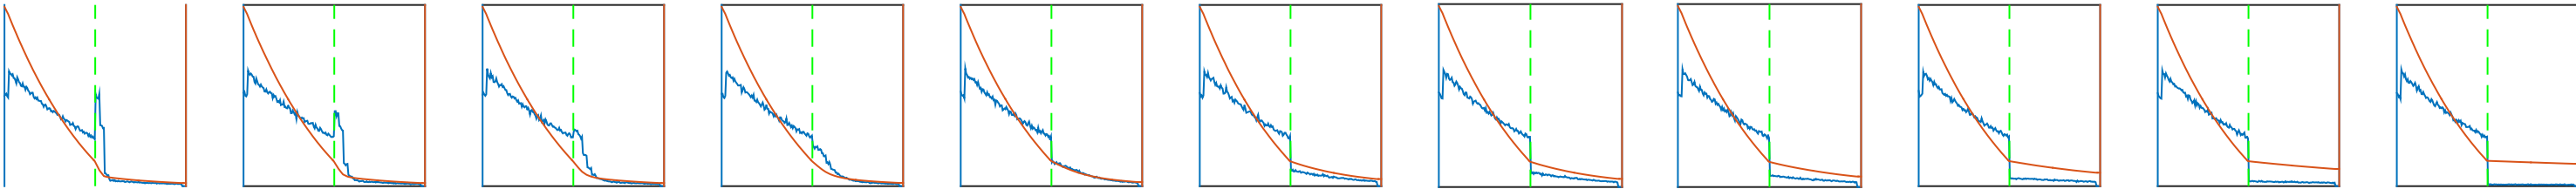

---

---

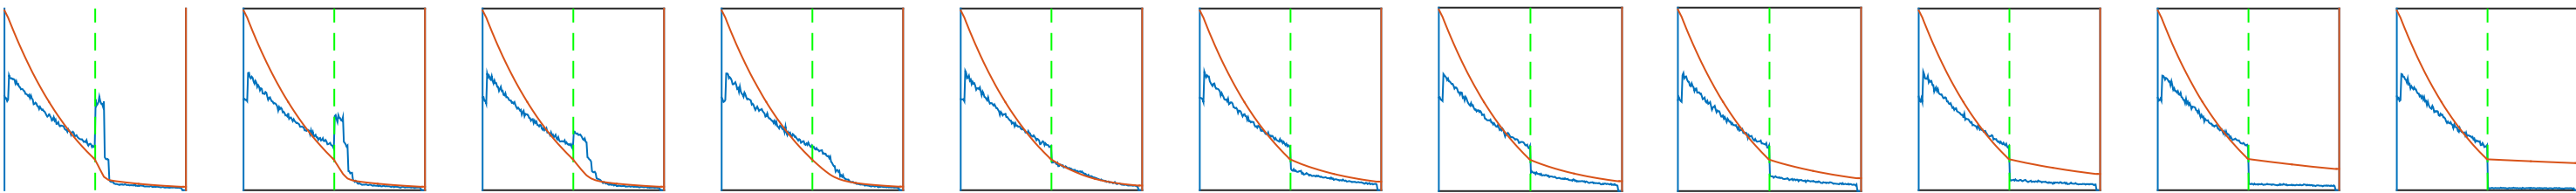

\_\_\_\_\_

\_\_\_\_\_

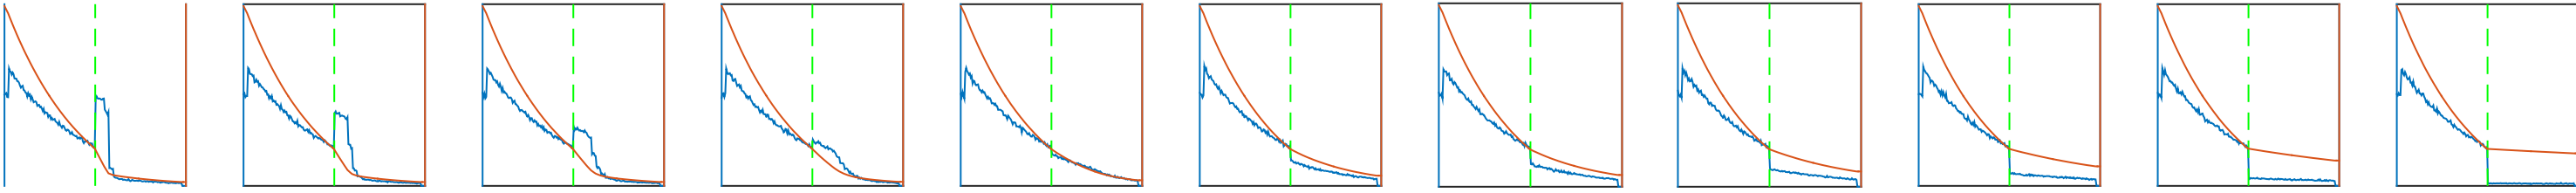

---

---

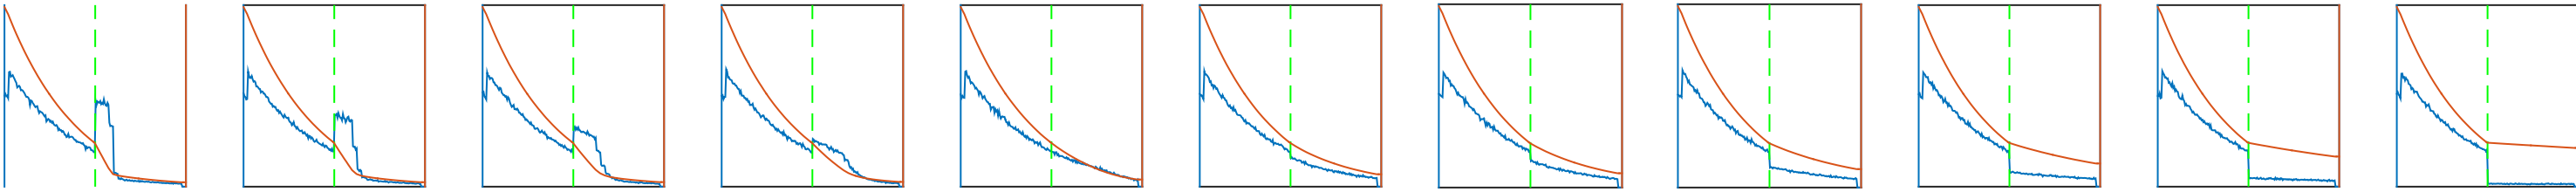

\_\_\_\_\_

\_\_\_\_\_

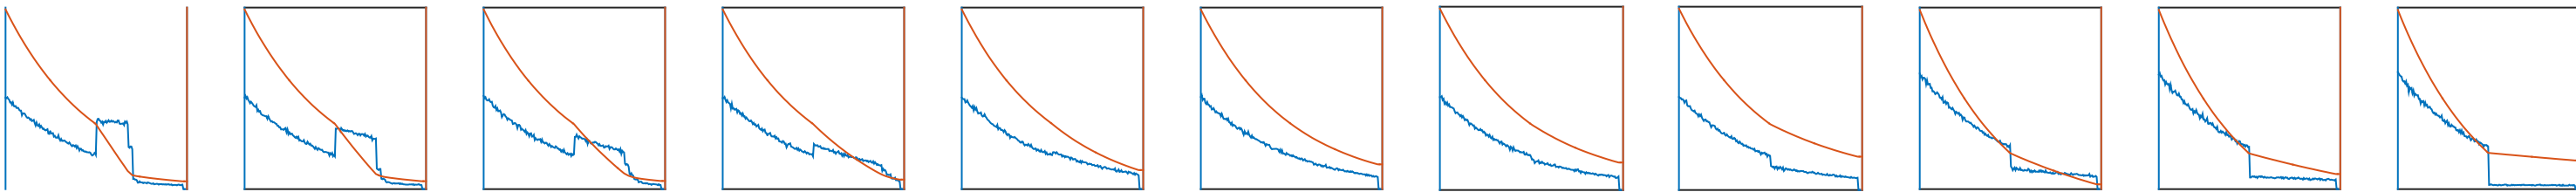

Supplement: Supplementary file 1 [file plot_boundaries_negative.pdf]
