# Supplementary material for: A Radiative Transfer Framework for Spatially-Correlated Materials
Source: arXiv:1805.02651 source file (2018-05-07)

---

---

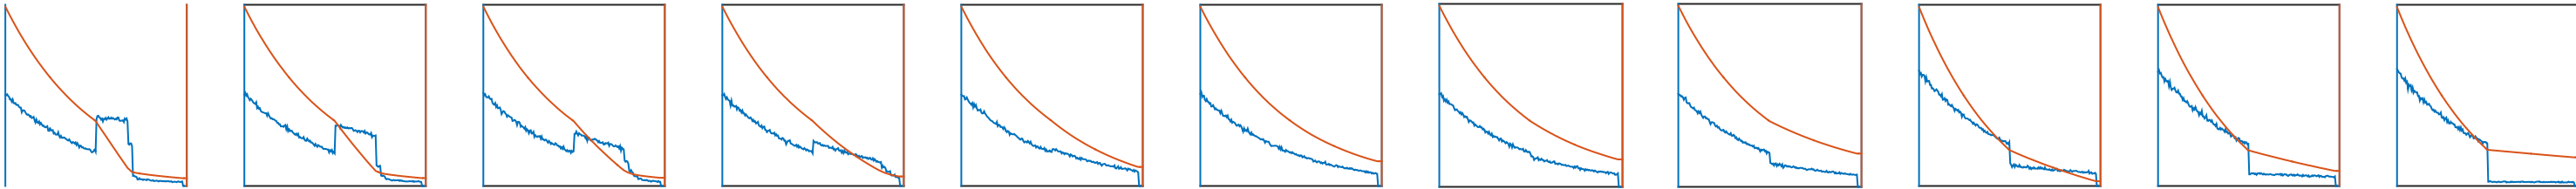

---

---

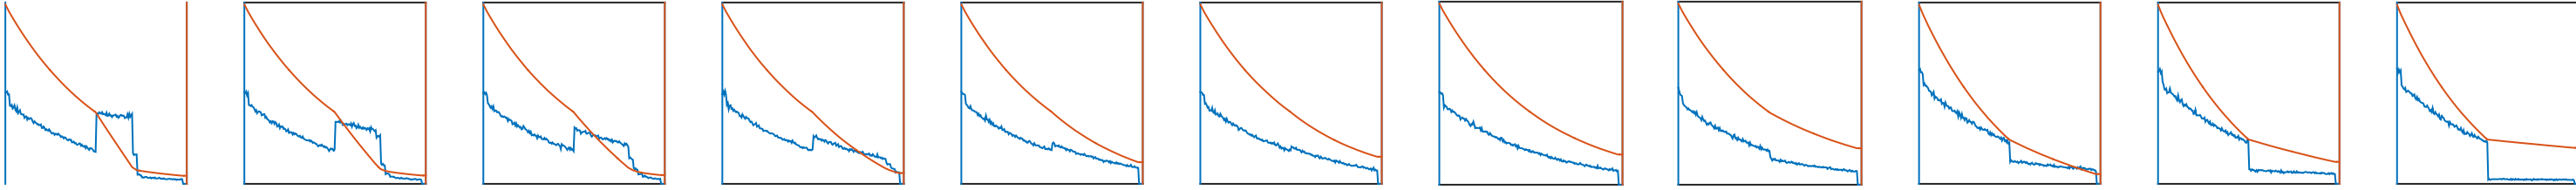

---

---

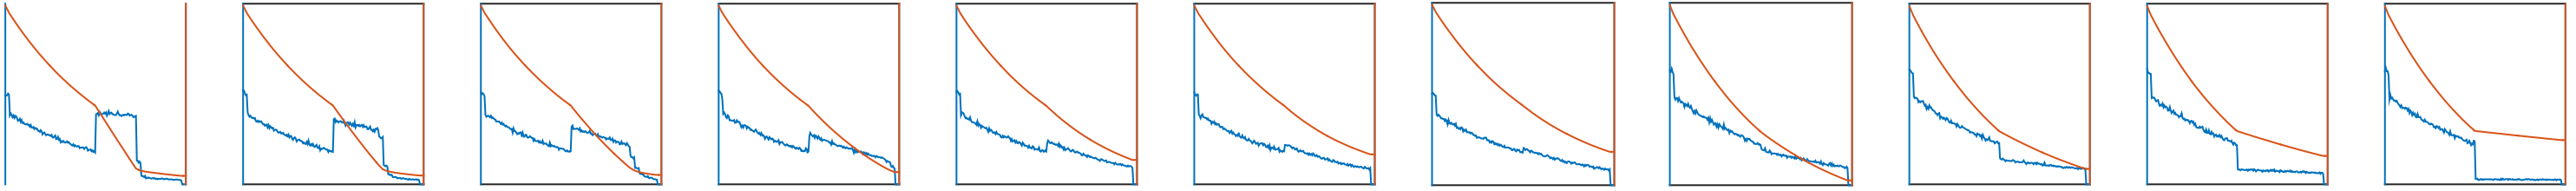

---

---

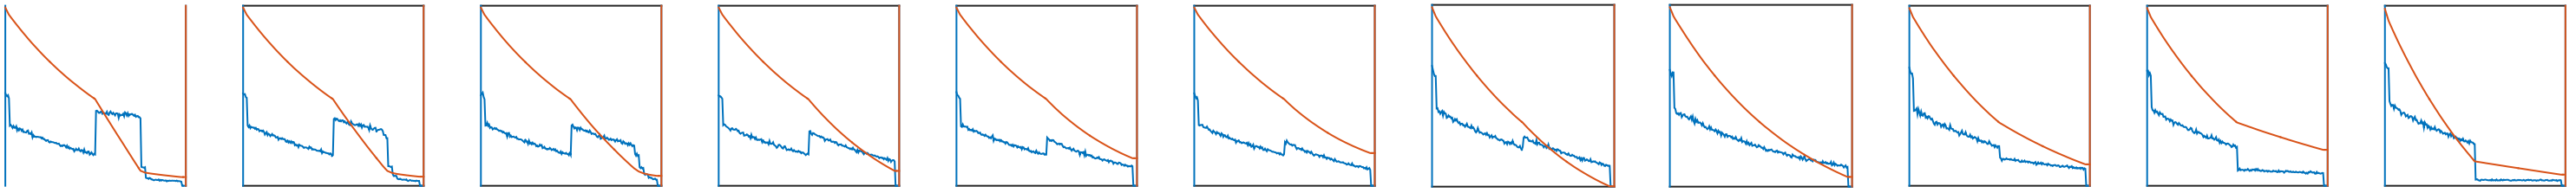

---

---

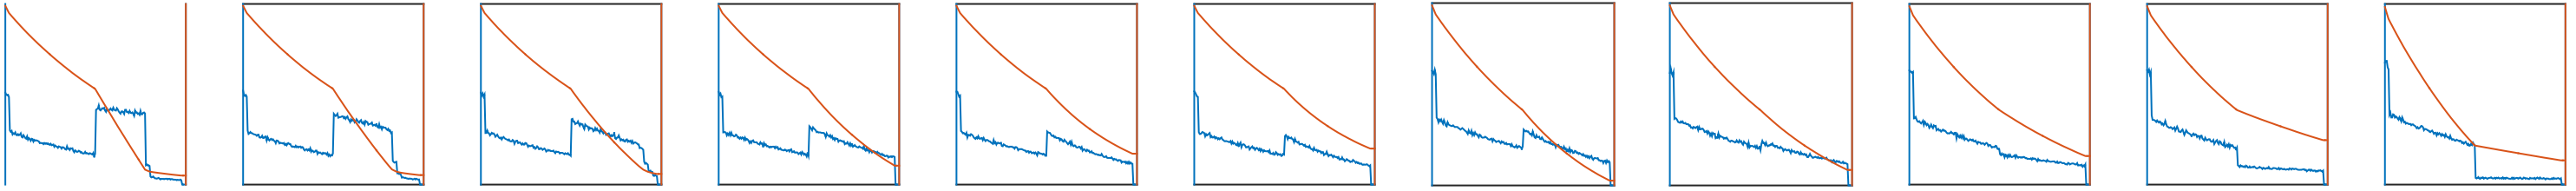

---

---

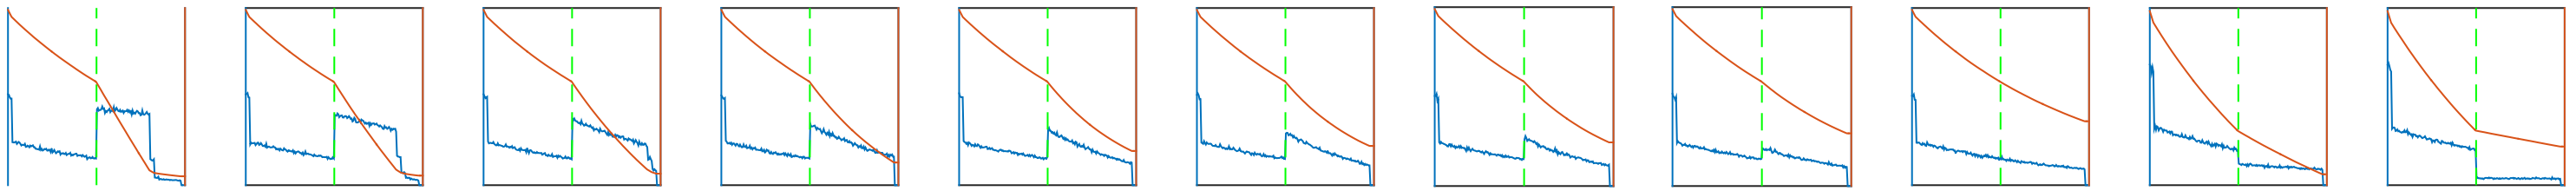

---

---

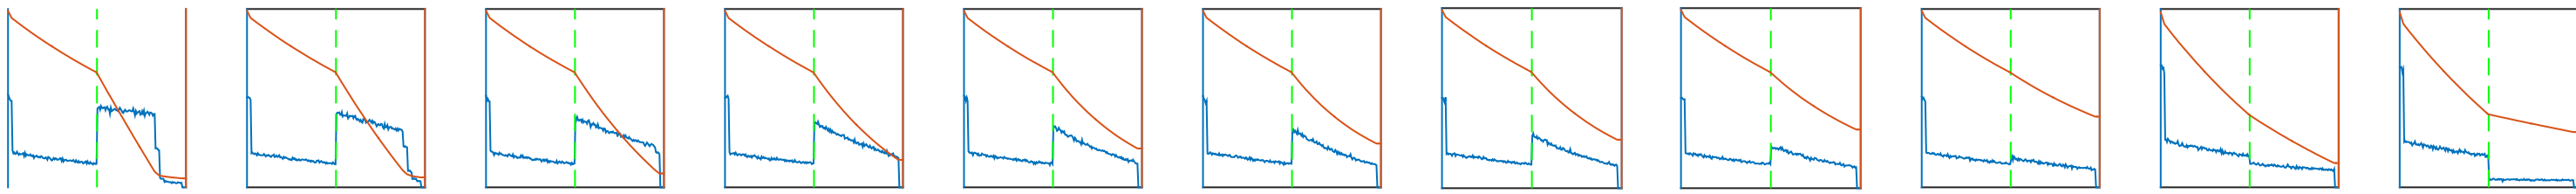

---

---



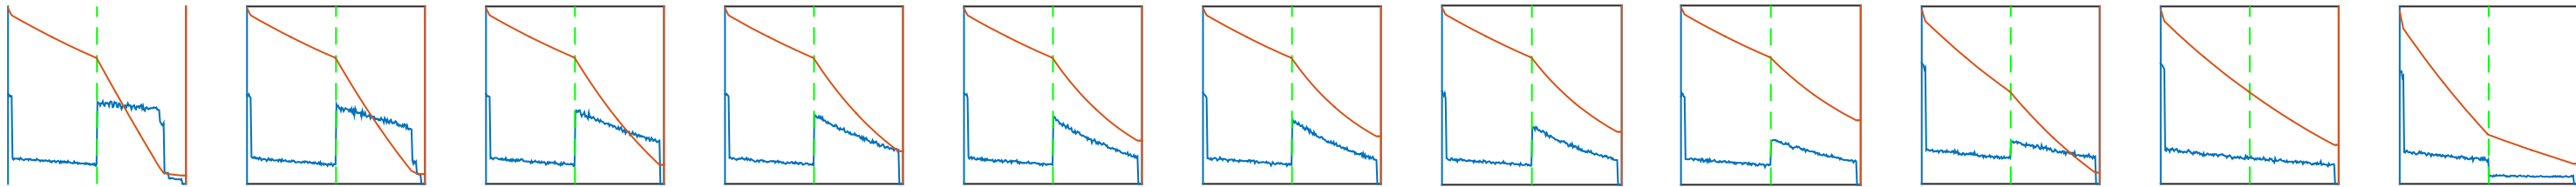

---

---

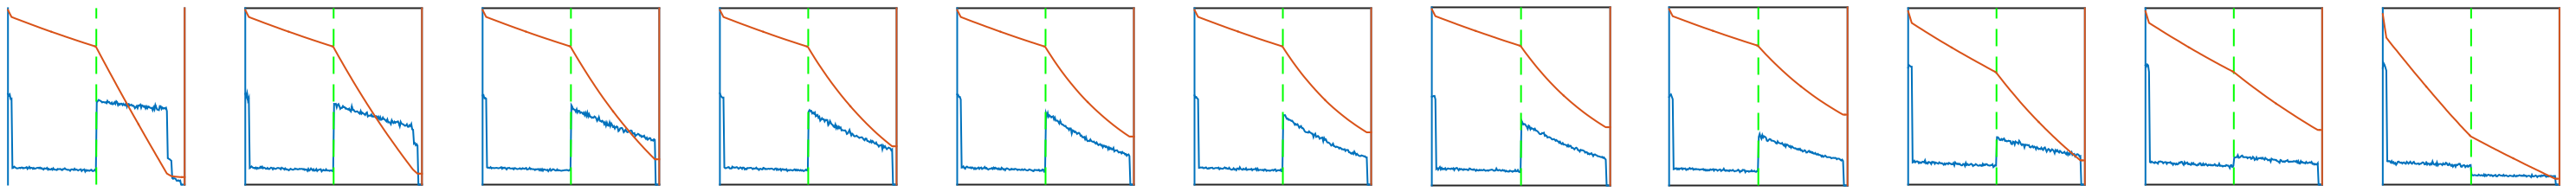



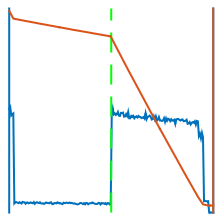



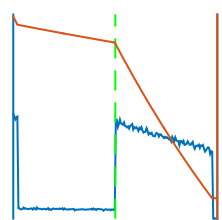



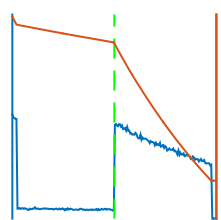





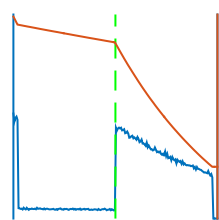



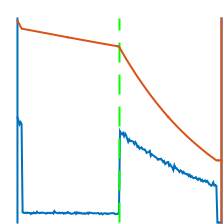



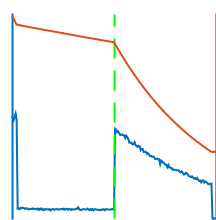



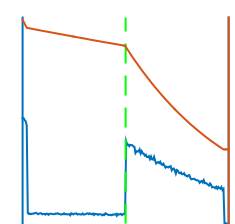





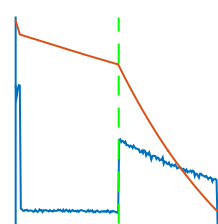



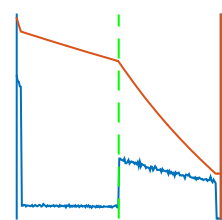



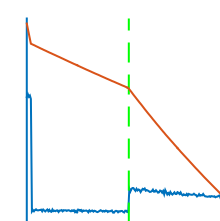



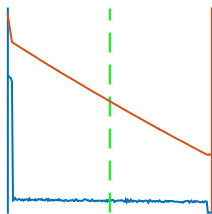

Supplement: Supplementary file 2 [file plot_boundaries_positive.pdf]
