# Supplementary material for: A Radiative Transfer Framework for Spatially-Correlated Materials
Source: arXiv:1805.02651 source file (2018-05-07)

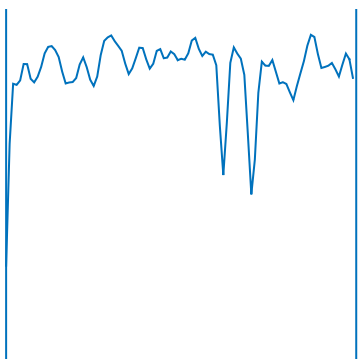

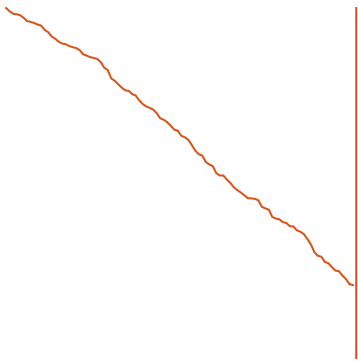



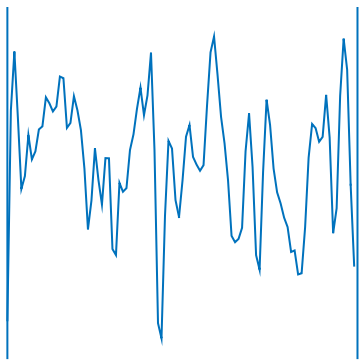

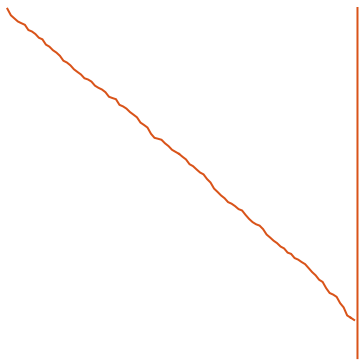





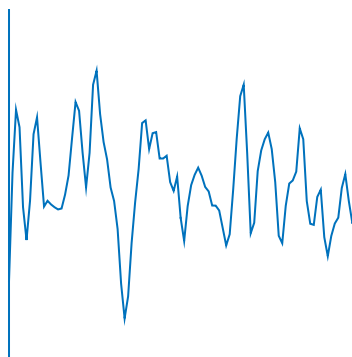

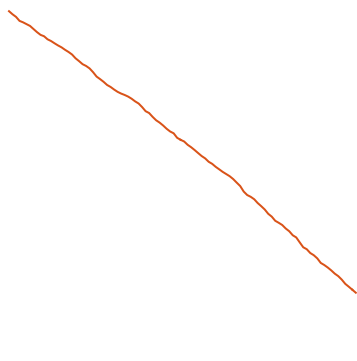



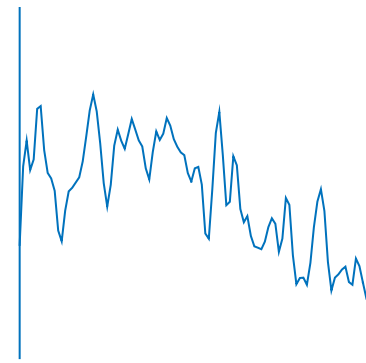





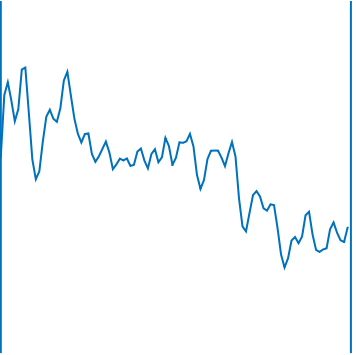





\_\_\_\_\_

\_\_\_\_\_

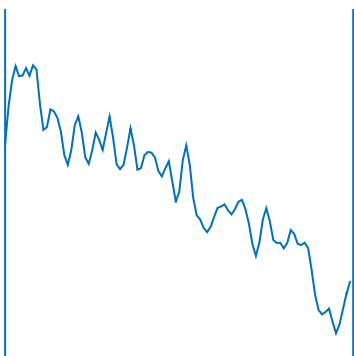

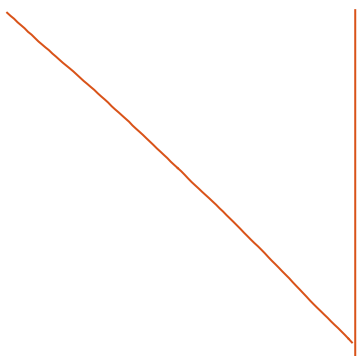

\_\_\_\_\_

\_\_\_\_\_

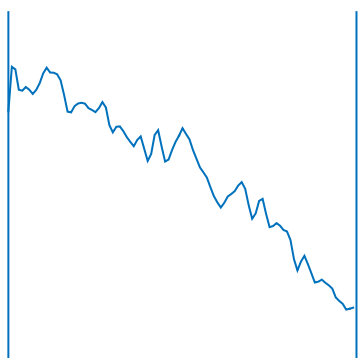

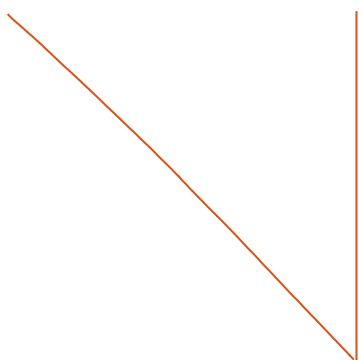

\_\_\_\_\_

\_\_\_\_\_

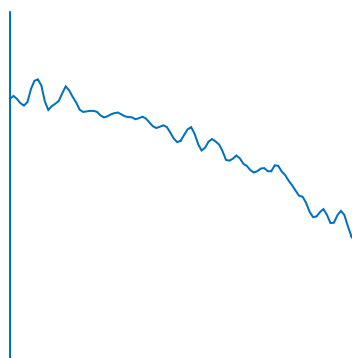



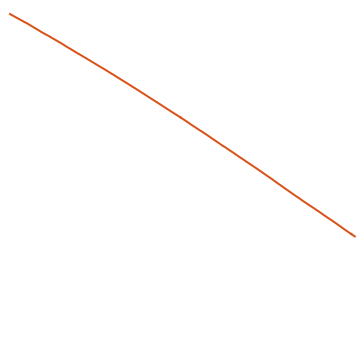

\_\_\_\_\_

\_\_\_\_\_

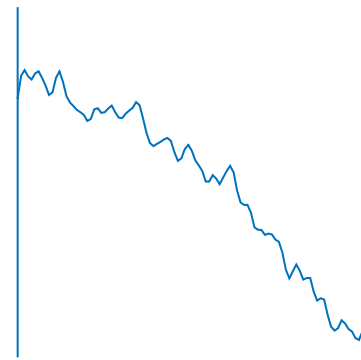



\_\_\_\_\_

\_\_\_\_\_

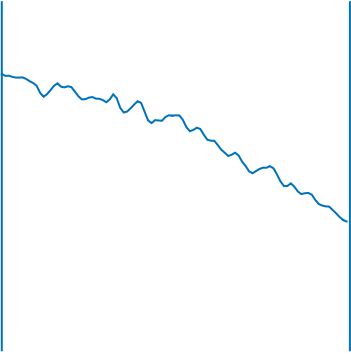

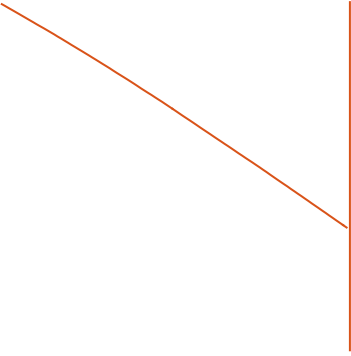

\_\_\_\_\_

\_\_\_\_\_



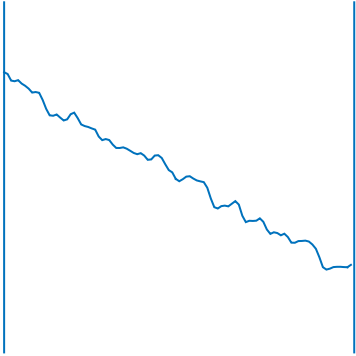



\_\_\_\_\_

\_\_\_\_\_

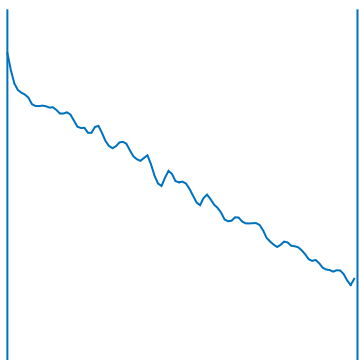

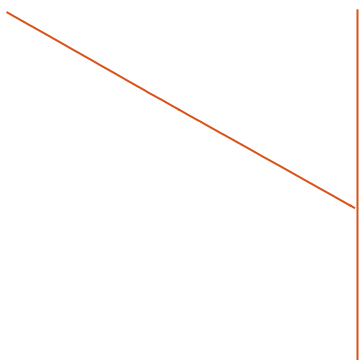

\_\_\_\_\_

\_\_\_\_\_

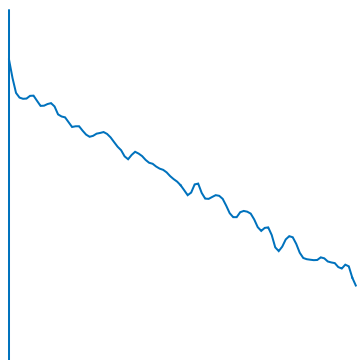

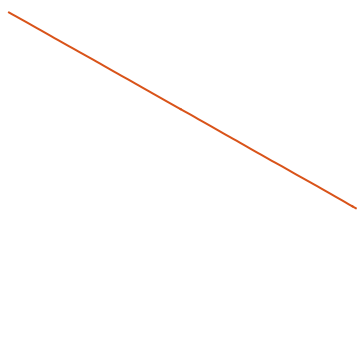



\_\_\_\_\_

\_\_\_\_\_

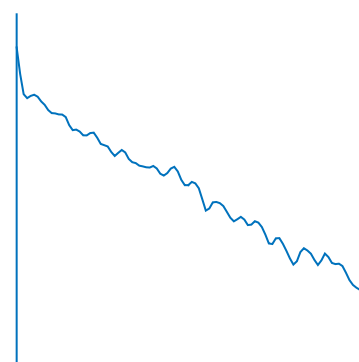



\_\_\_\_\_

\_\_\_\_\_

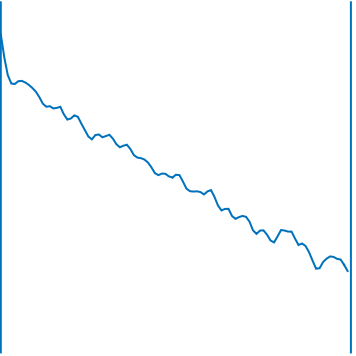



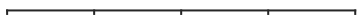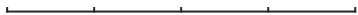

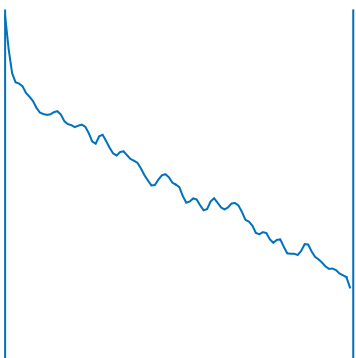





\_\_\_\_\_

\_\_\_\_\_

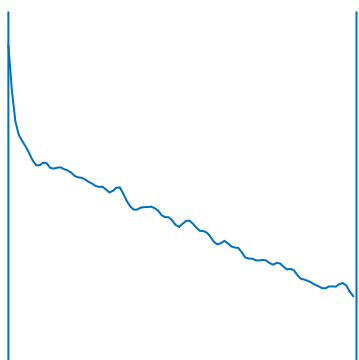

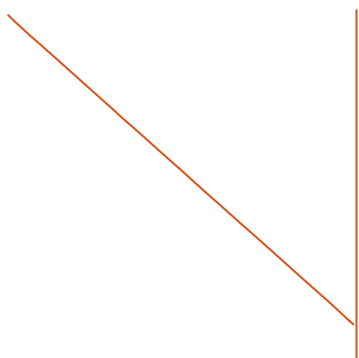

\_\_\_\_\_

\_\_\_\_\_

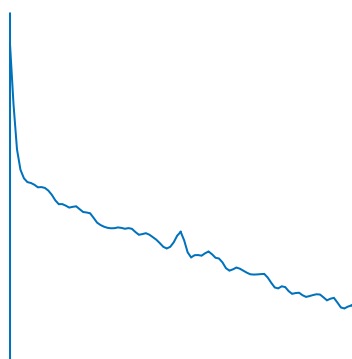

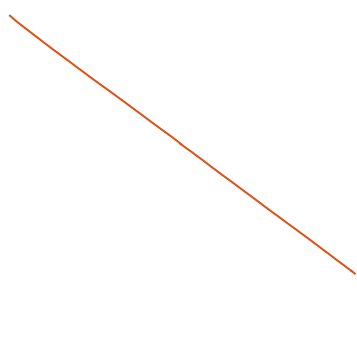

\_\_\_\_\_

\_\_\_\_\_



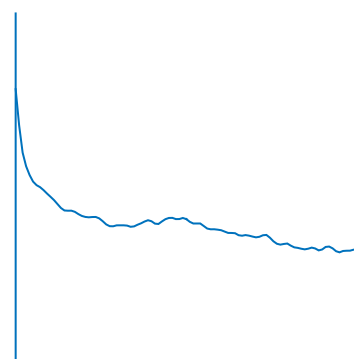

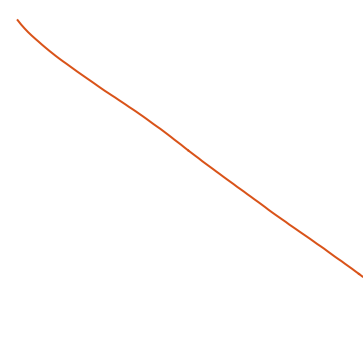

\_\_\_\_\_

\_\_\_\_\_

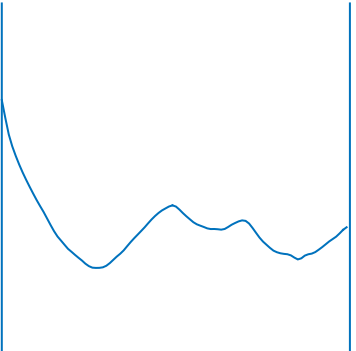

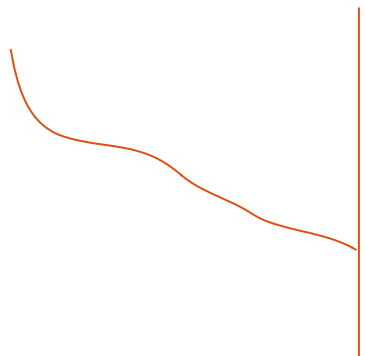

Supplement: Supplementary file 3 [file plot_inscattering.pdf]
