# Supplementary material for: A Radiative Transfer Framework for Spatially-Correlated Materials
Source: arXiv:1805.02651 source file (2018-05-07)
Supplement: Supplementary file 4 [file plot_source.pdf]

\_\_\_\_\_

\_\_\_\_\_



||



\_\_\_\_\_

\_\_\_\_\_

N

\_\_\_\_\_

\_\_\_\_\_





\_\_\_\_\_

\_\_\_\_\_

N

\_\_\_\_\_

\_\_\_\_\_



\_\_\_\_\_

\_\_\_\_\_

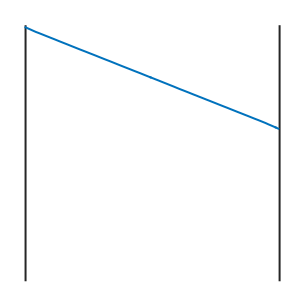

\_\_\_\_\_

\_\_\_\_\_



N

\_\_\_\_\_

\_\_\_\_\_



\_\_\_\_\_

\_\_\_\_\_

N

\_\_\_\_\_

\_\_\_\_\_



[

]





\_\_\_\_\_

\_\_\_\_\_

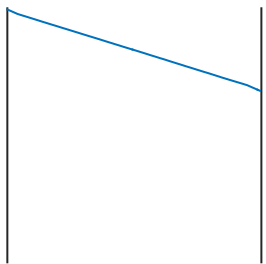

\_\_\_\_\_

\_\_\_\_\_



\_\_\_\_\_

\_\_\_\_\_

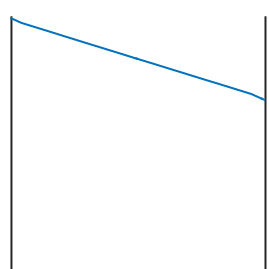

\_\_\_\_\_

\_\_\_\_\_





\_\_\_\_\_

\_\_\_\_\_

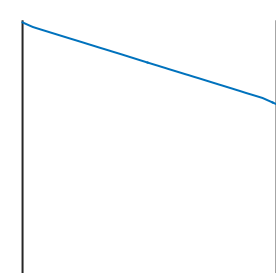

\_\_\_\_\_

\_\_\_\_\_

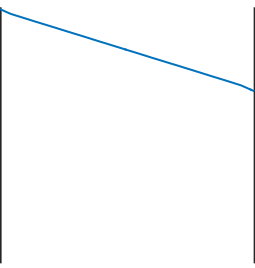

\_\_\_\_\_

\_\_\_\_\_



\_\_\_\_\_

\_\_\_\_\_



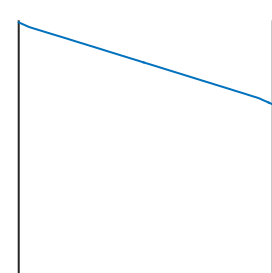

\_\_\_\_\_

\_\_\_\_\_



||



\_\_\_\_\_

\_\_\_\_\_

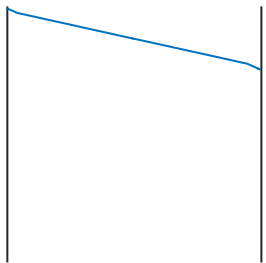

\_\_\_\_\_

\_\_\_\_\_





\_\_\_\_\_

\_\_\_\_\_

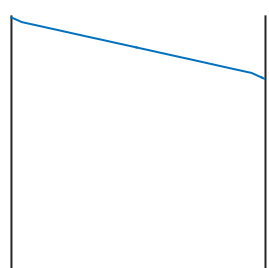

\_\_\_\_\_

\_\_\_\_\_



\_\_\_\_\_

\_\_\_\_\_

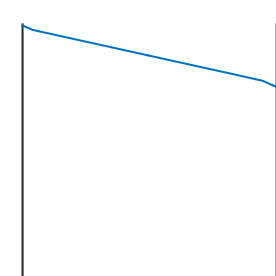

\_\_\_\_\_

\_\_\_\_\_



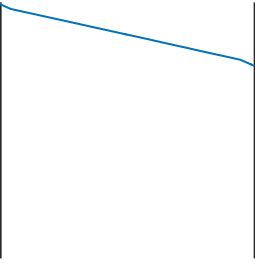

\_\_\_\_\_

\_\_\_\_\_



\_\_\_\_\_

\_\_\_\_\_

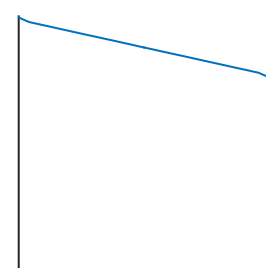

\_\_\_\_\_

\_\_\_\_\_



[

]





---

---

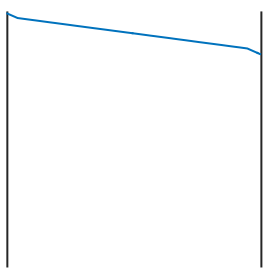

\_\_\_\_\_

\_\_\_\_\_



\_\_\_\_\_

\_\_\_\_\_

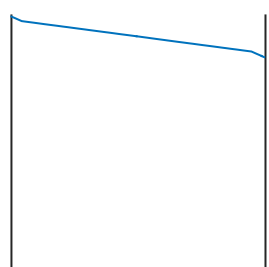

\_\_\_\_\_

\_\_\_\_\_





\_\_\_\_\_

\_\_\_\_\_

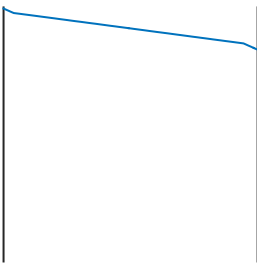

\_\_\_\_\_

\_\_\_\_\_

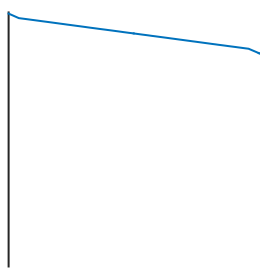

\_\_\_\_\_

\_\_\_\_\_



\_\_\_\_\_

\_\_\_\_\_



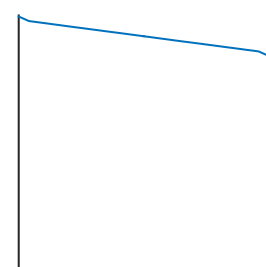





|

|





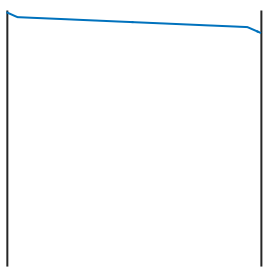





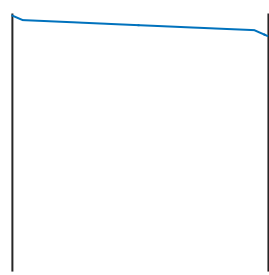



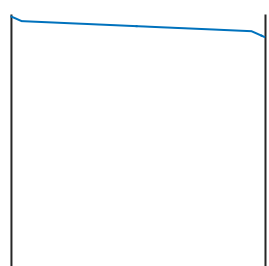



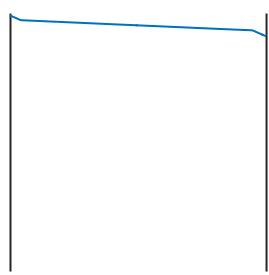



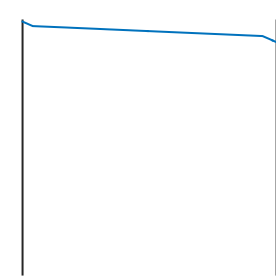





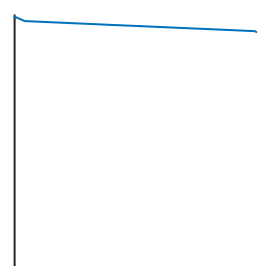



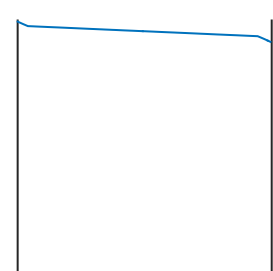



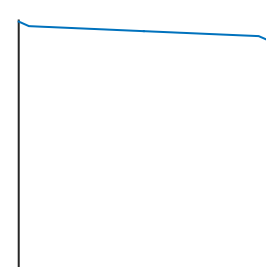

\_\_\_\_\_

\_\_\_\_\_



||





\_\_\_\_\_

\_\_\_\_\_



\_\_\_\_\_

\_\_\_\_\_

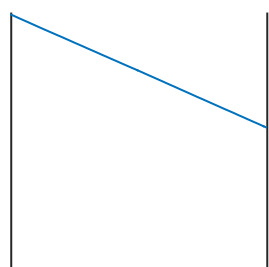

\_\_\_\_\_

\_\_\_\_\_

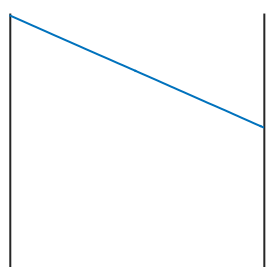

\_\_\_\_\_

\_\_\_\_\_



N

\_\_\_\_\_

\_\_\_\_\_

N

\_\_\_\_\_

\_\_\_\_\_

N

\_\_\_\_\_

\_\_\_\_\_

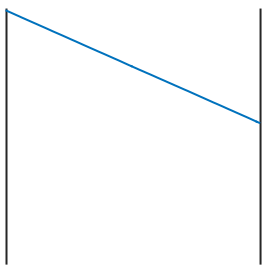

\_\_\_\_\_

\_\_\_\_\_



N





|

|







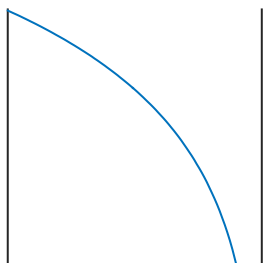













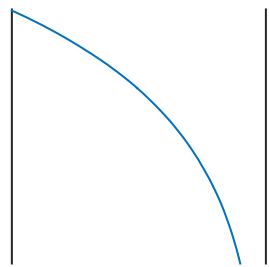







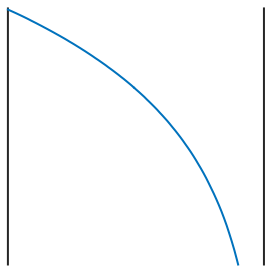











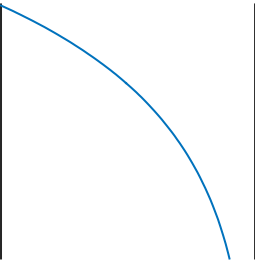













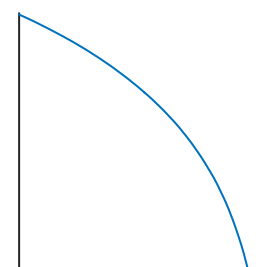



\_\_\_\_\_

\_\_\_\_\_





||



\_\_\_\_\_

\_\_\_\_\_

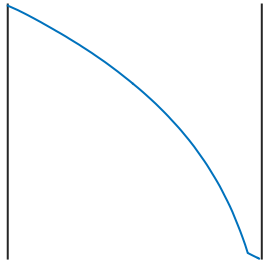





\_\_\_\_\_

\_\_\_\_\_

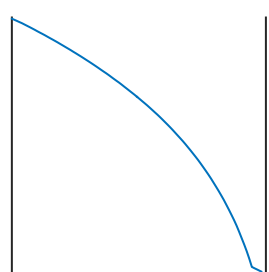





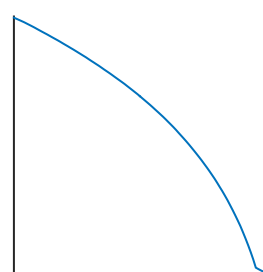

\_\_\_\_\_

\_\_\_\_\_



\_\_\_\_\_

\_\_\_\_\_

N

\_\_\_\_\_

\_\_\_\_\_





\_\_\_\_\_

\_\_\_\_\_

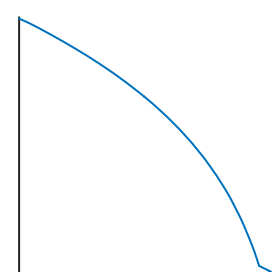





|

|





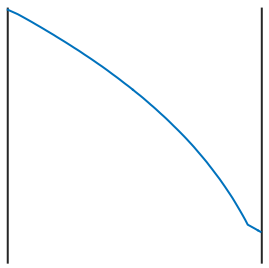









N



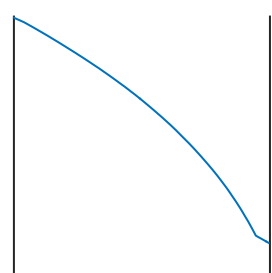









N







N







||





N







N





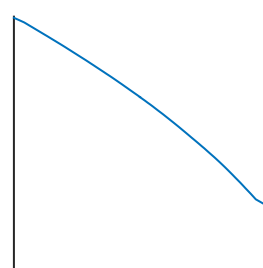







N









N





||





N



\_\_\_\_\_

\_\_\_\_\_





N

\_\_\_\_\_

\_\_\_\_\_

N









N







N
